# Supplementary material for: Fast Algorithms for the computation of Fourier Extensions of arbitrary length
Source: arXiv:1509.00206 source file (2015-09-01)
Supplement: Supplementary file 1 [file appendix.tex]

% !TEX root = paper1.tex
\appendix
\label{app:theoremproof}
\section{Proof of Theorem \ref{thm:mapping}}
\begin{proof}
First we note a similar result from the continuous Fourier Extension. Let $\CM$ be the matrix of the continuous FE with eigenvalues $\bar{\sigma}_i$, and $\bar{T}$ the tridiagonal matrix (\ref{eqn:barTtridiag}) with eigenvalues $\bar{\theta}_i$. Then define the mapping $\bar{\mathcal{G}}$ by
\begin{equation*}
j=\bar{\mathcal{G}}(i)\Leftrightarrow\begin{cases}\phi_i'\bar{T}\phi_i=\bar{\theta}_j&\\
\phi_i'\CM\phi_i=\bar{\sigma}_i & \end{cases},
\end{equation*}
where the $\phi_i$ are DPSSs. The mapping $\bar{\mathcal{G}}$ was proven to be order-preserving in \cite{Slepian1978a}.

Then we look at the limits of the entries of $\DM'\DM$ and $T_{N,M}$ for large $\sm$:
\begin{align*}
\lim_{\sm\to\infty}(\DM'\DM)_{ij}&=\frac{\sin{\frac{(i-j)\pi}{T}}}{\pi(i-j)}=\CM_{ij}\\
\lim_{\sm\to\infty}b_k&=\frac{\pi^2k(N-k)}{L^2}=\frac{2\pi^2}{L^2}\bar{b}_k\\
\lim_{\sm\to\infty}c_k&=\cos{\frac{\pi}{T}}\left(\frac{2\pi^2}{L^2}\left(\frac{N-1}{2}-k\right)^2-1\right)=\frac{2\pi^2}{L^2}\bar{c}_k-\cos{\frac{\pi}{T}}
\end{align*}
Apart from the factor $\frac{L^2}{2\pi^2}$ and the additional diagonal term $\frac{L^2}{2\pi^2}\cos{\frac{\pi}{T}}$, the entries are similar to those for the DPSS problem. Since these changes don't influence the ordering of the eigenvalues, the theorem is now shown to hold in the limit $m\to\infty$.

Further, since \pdfcomment{The eigenvalue reasoning hold for Jacobi and in general Symmetric matrices. The eigenvector reasoning is unproven. Also the proof will only hold for $m$ large enough to avoid degenerate eigenvalues.}
\begin{itemize}
\item The eigenvalues and eigenvectors of $T_{N,M}$ are distinct and continuous in $\forall\sm>\sn$.
\item The eigenvalues and eigenvectors of $\DM$ are distinct and continuous $\forall\sm>\sn$.
\end{itemize}
the theorem is valid for all $\sm>\sn$.
\end{proof}
